# Supplementary material for: Improving 2D Diffusion Models for 3D Medical Imaging with Inter-Slice Consistent Stochasticity
Source: arXiv:2602.04162 source file (2026-02-09)
Supplement: Supplementary file 1 [file Appendix_fig_simulate_SVCT.pdf]

Axial

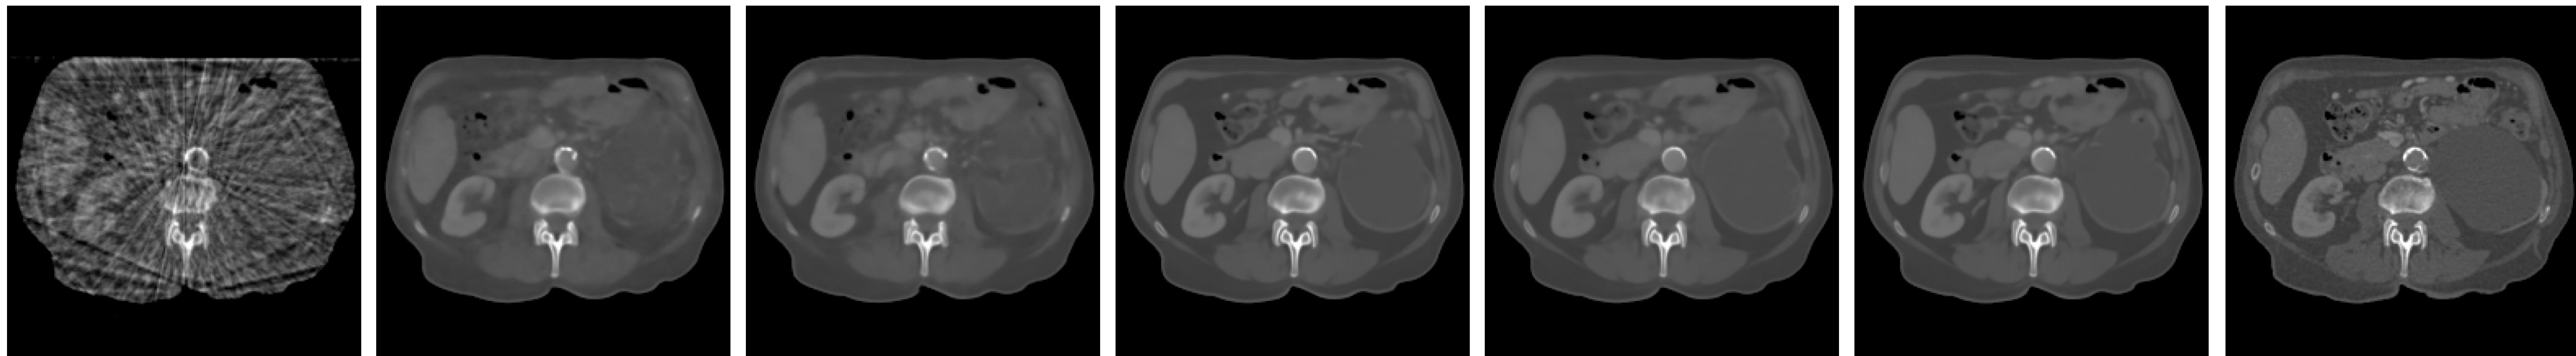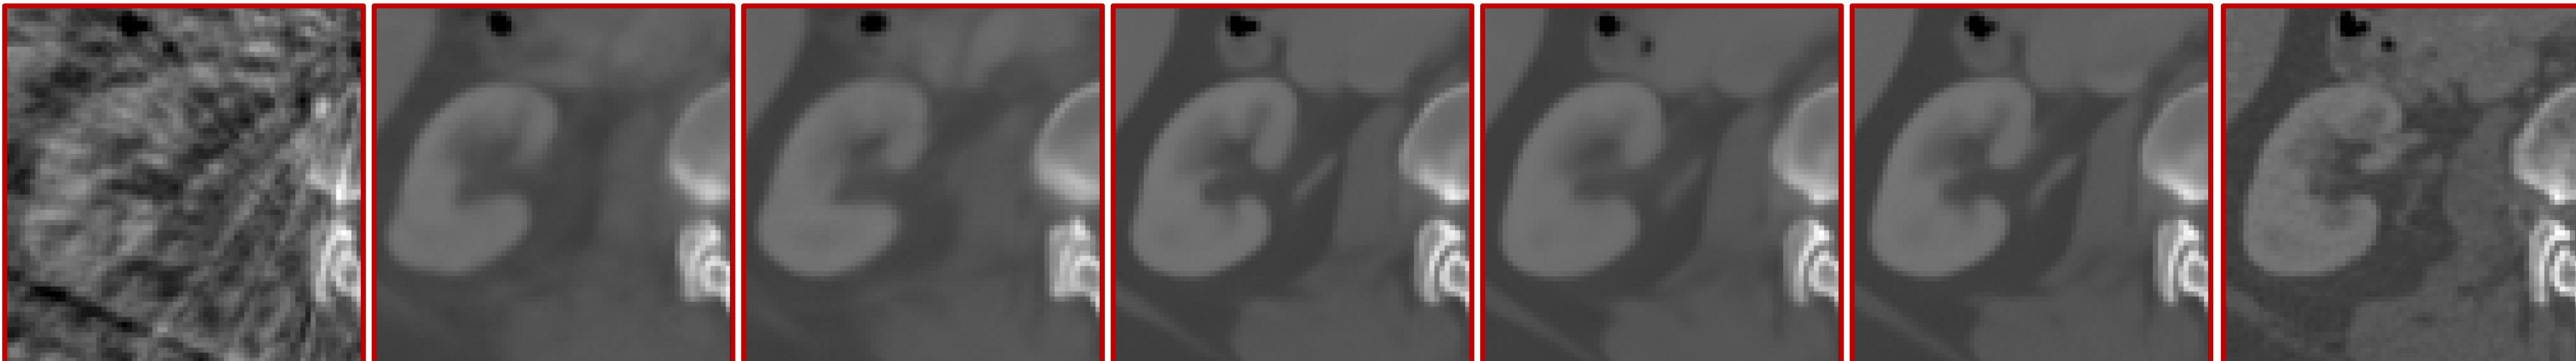

Sagittal

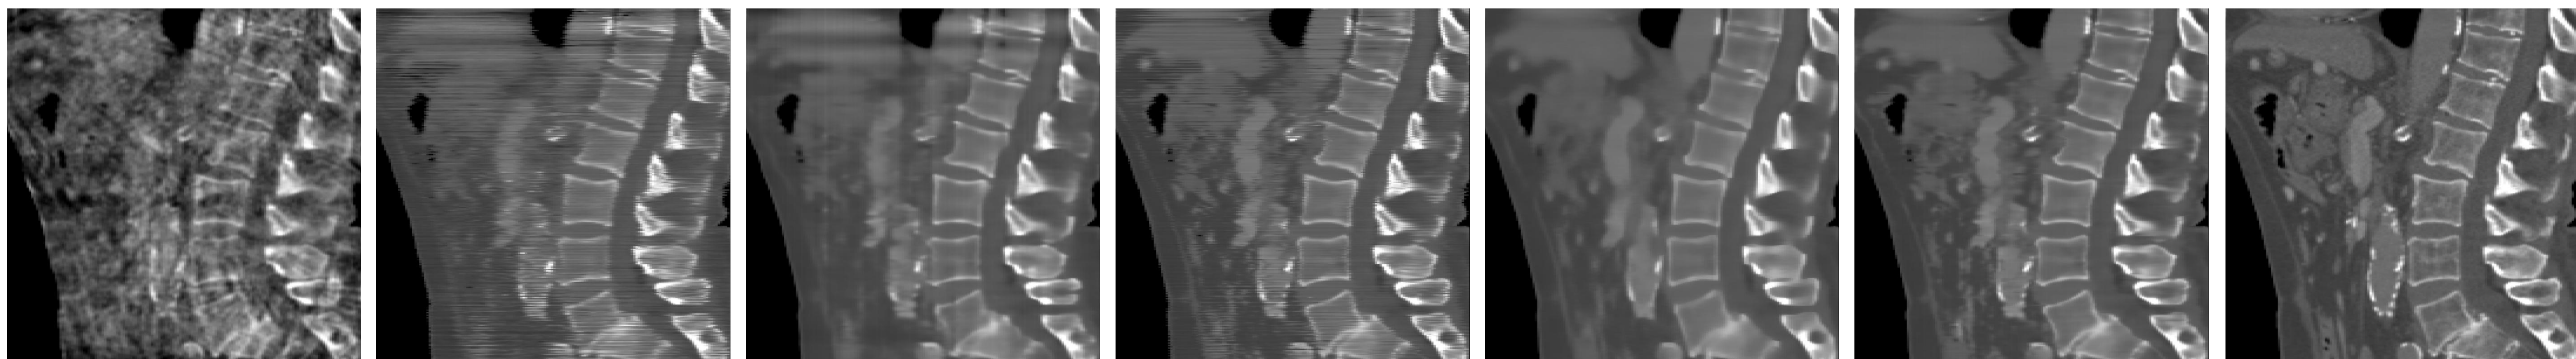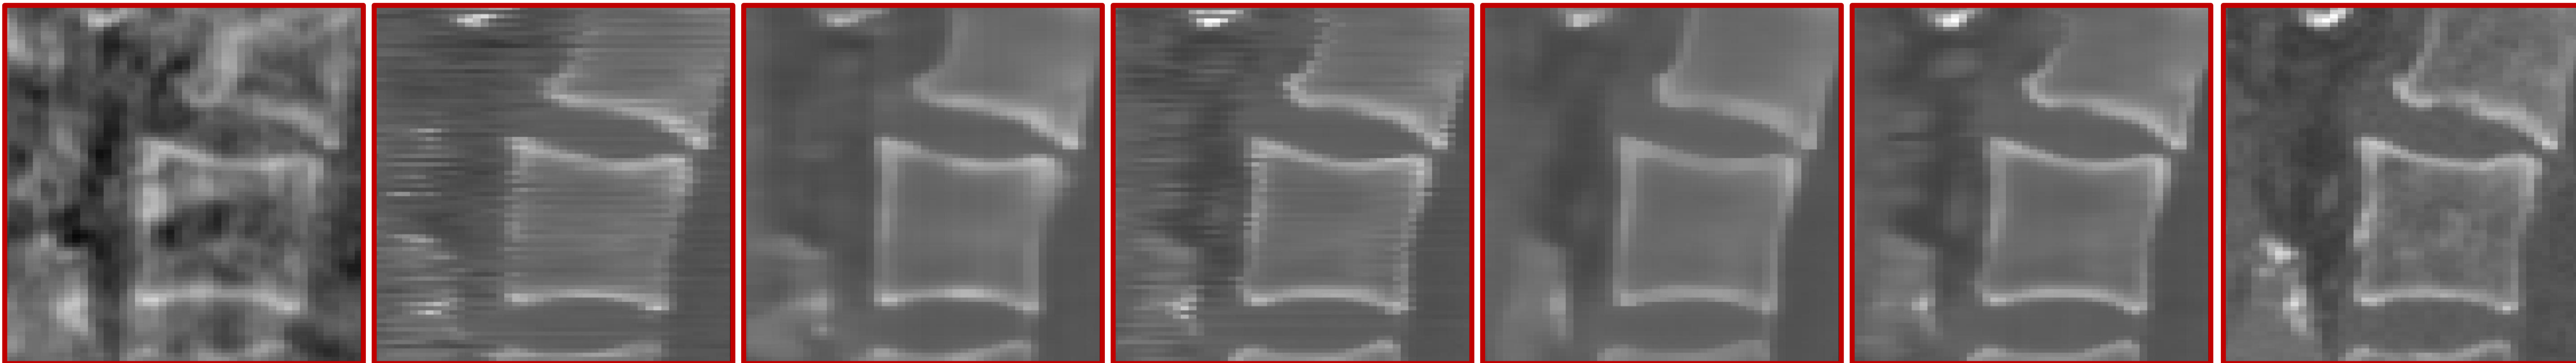

Coronal

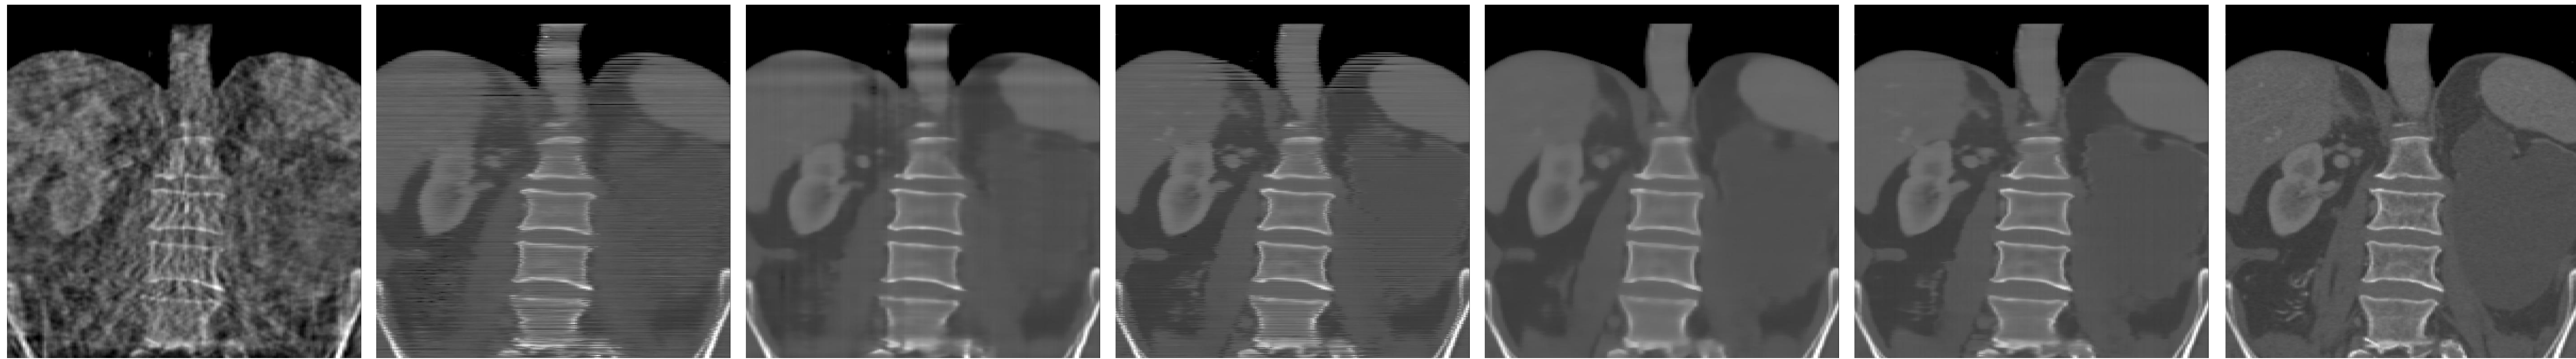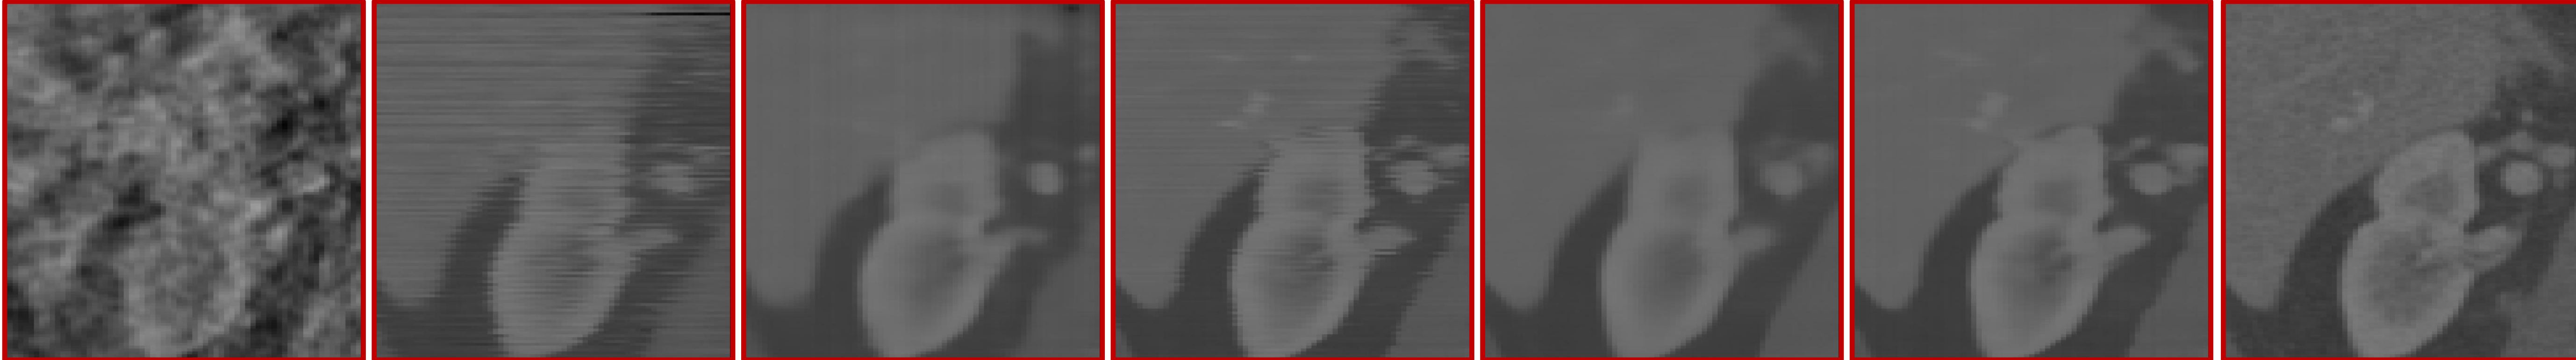

FDK

DDNM

DDNM+ISCS

DDS

DDS+TV

DDS+ISCS

GT



Axial

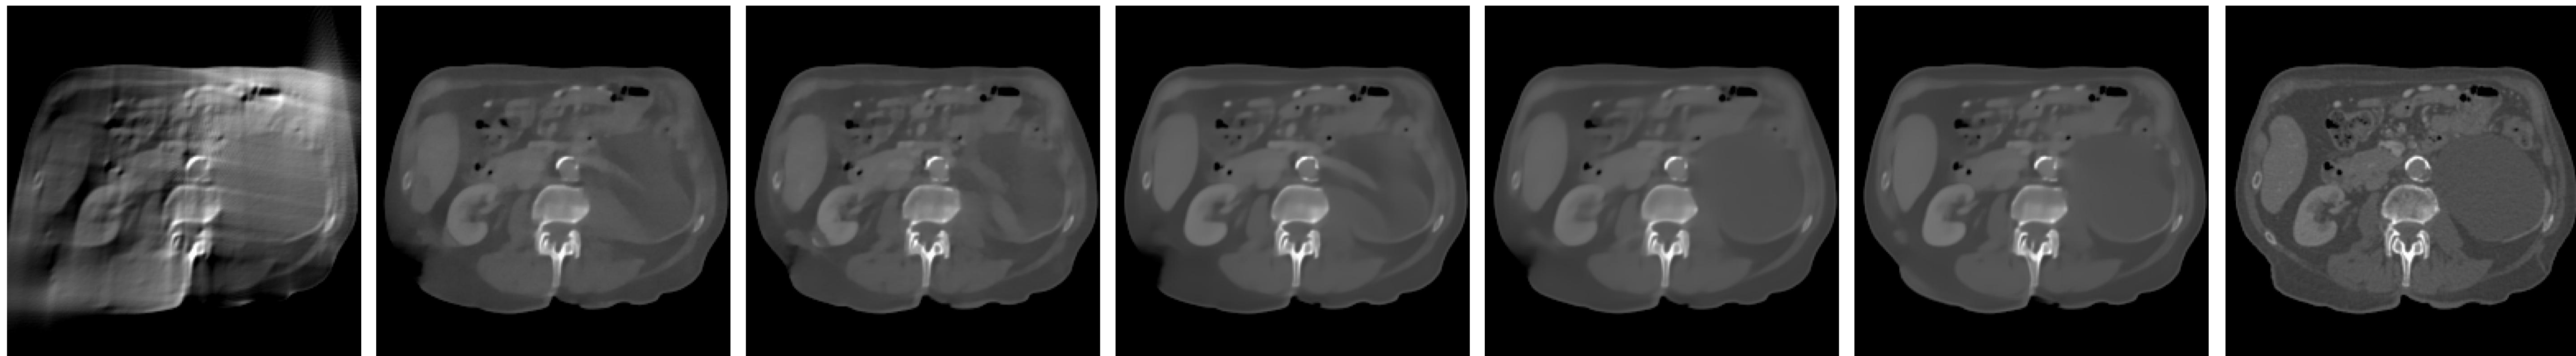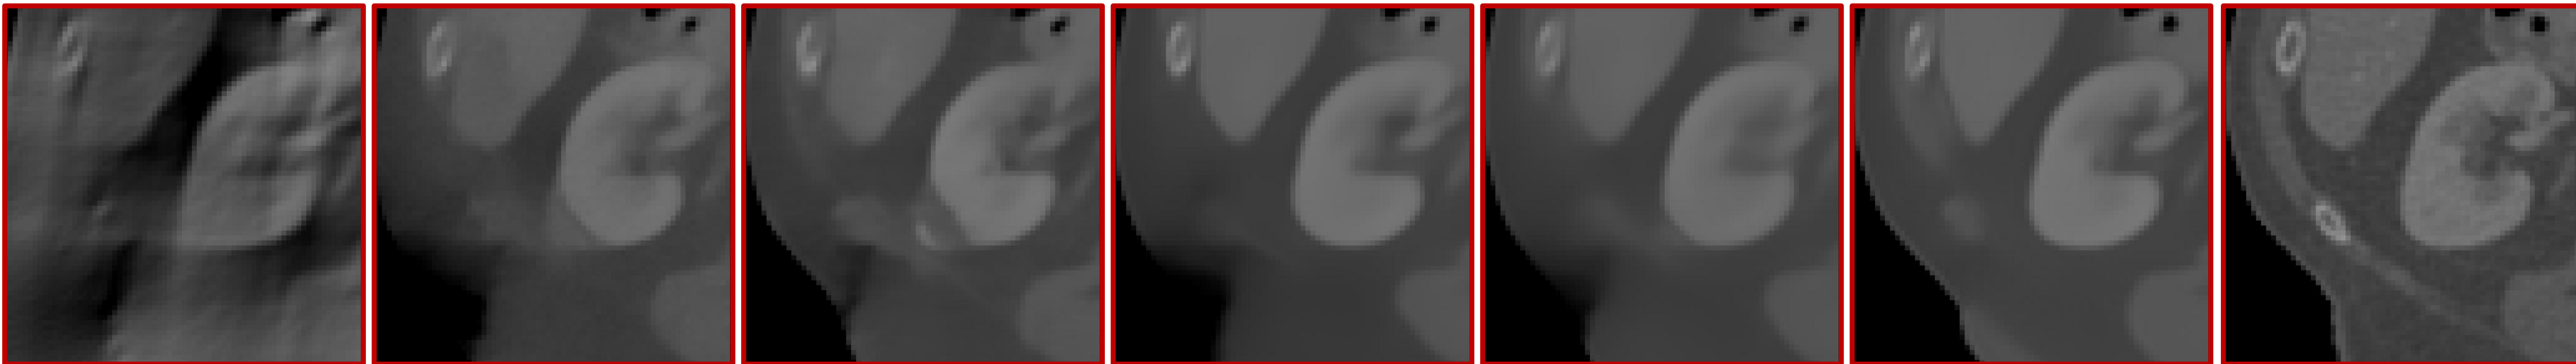

Sagittal

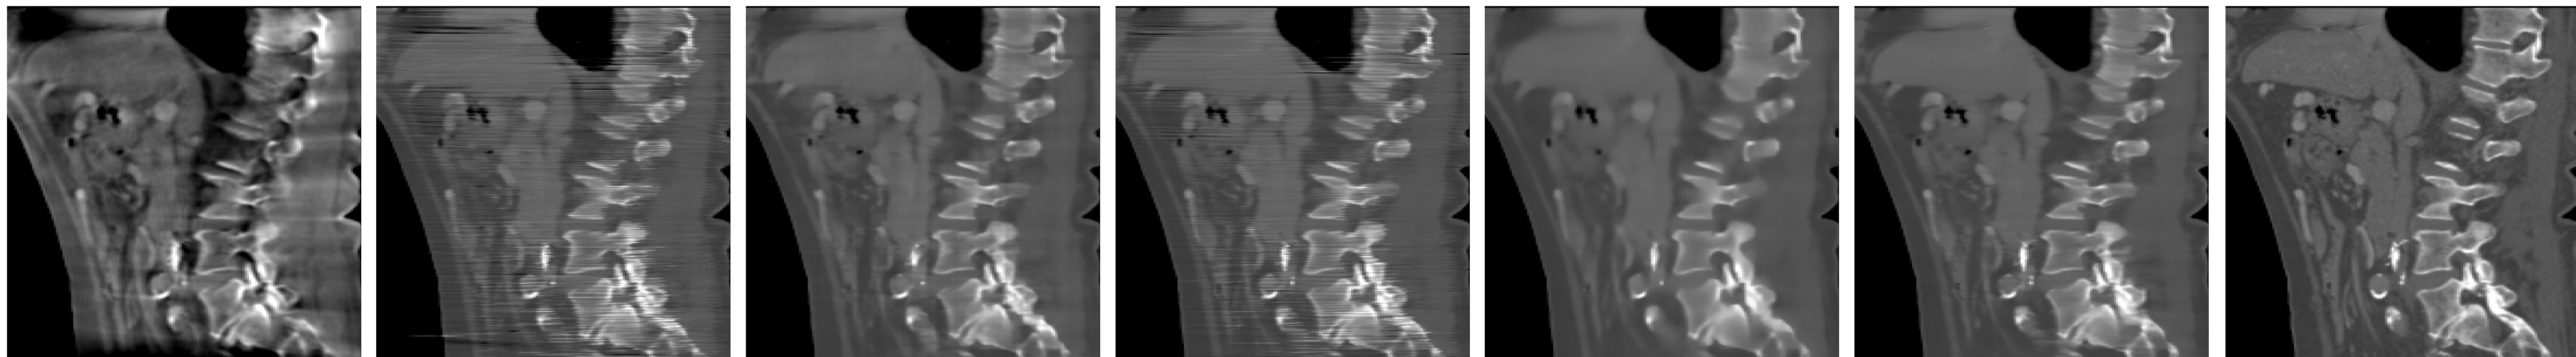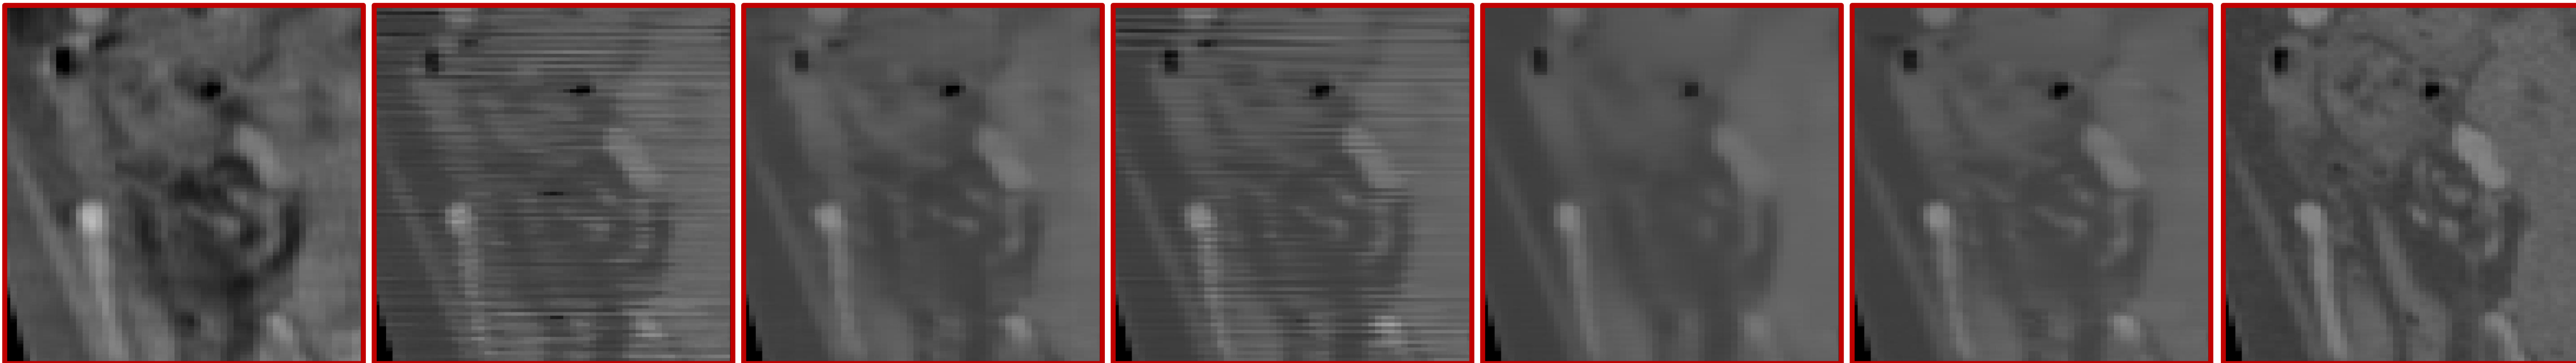

Coronal

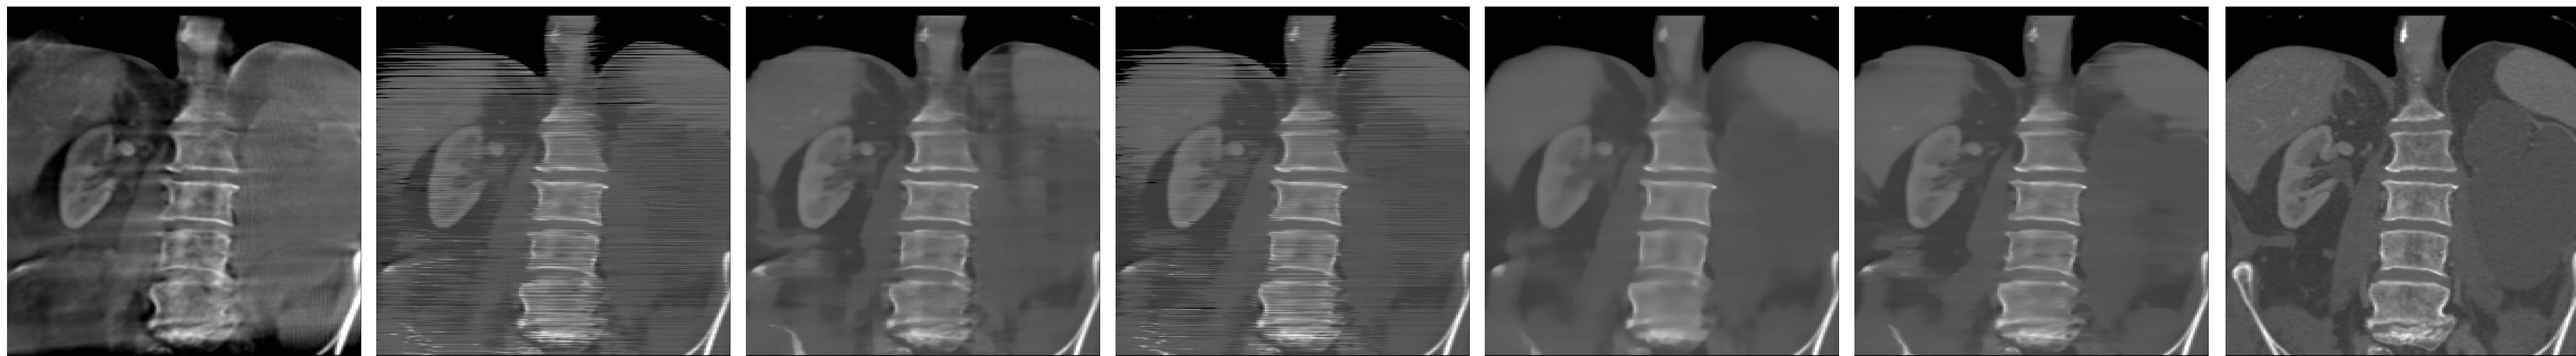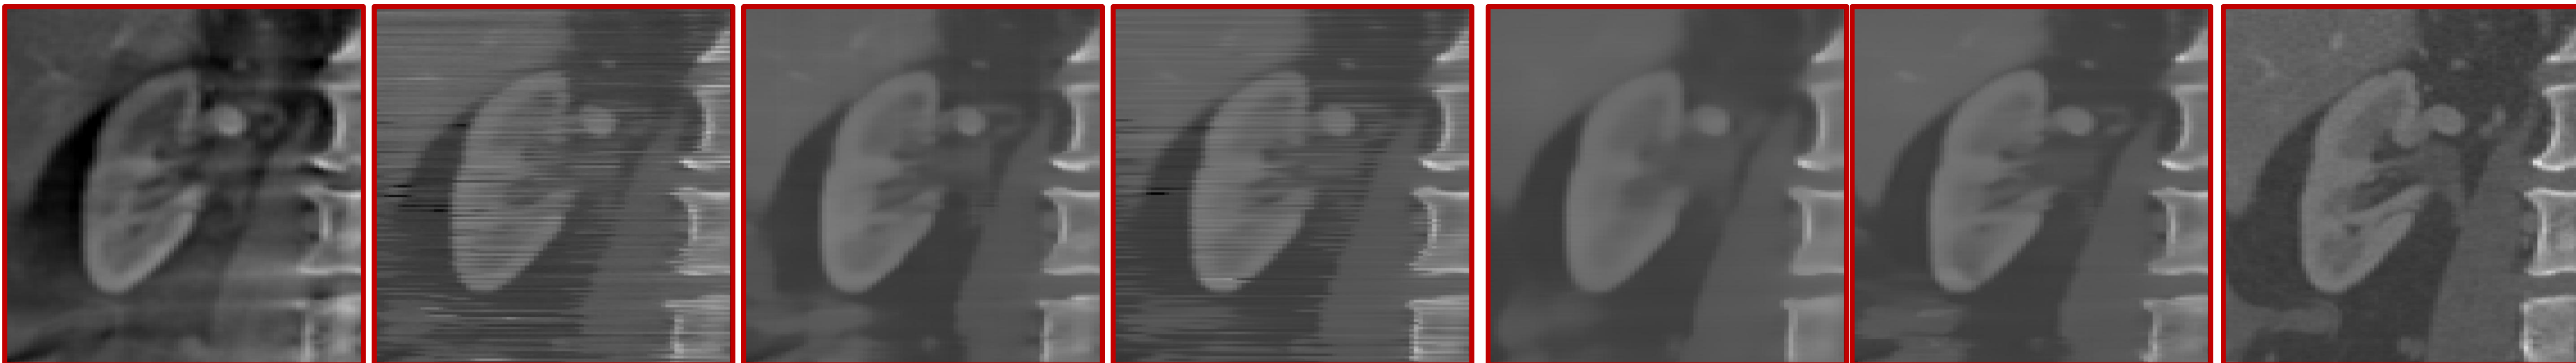

FDK

DDNM

DDNM+ISCS

DDS

DDS+TV

DDS+ISCS

GT



Axial

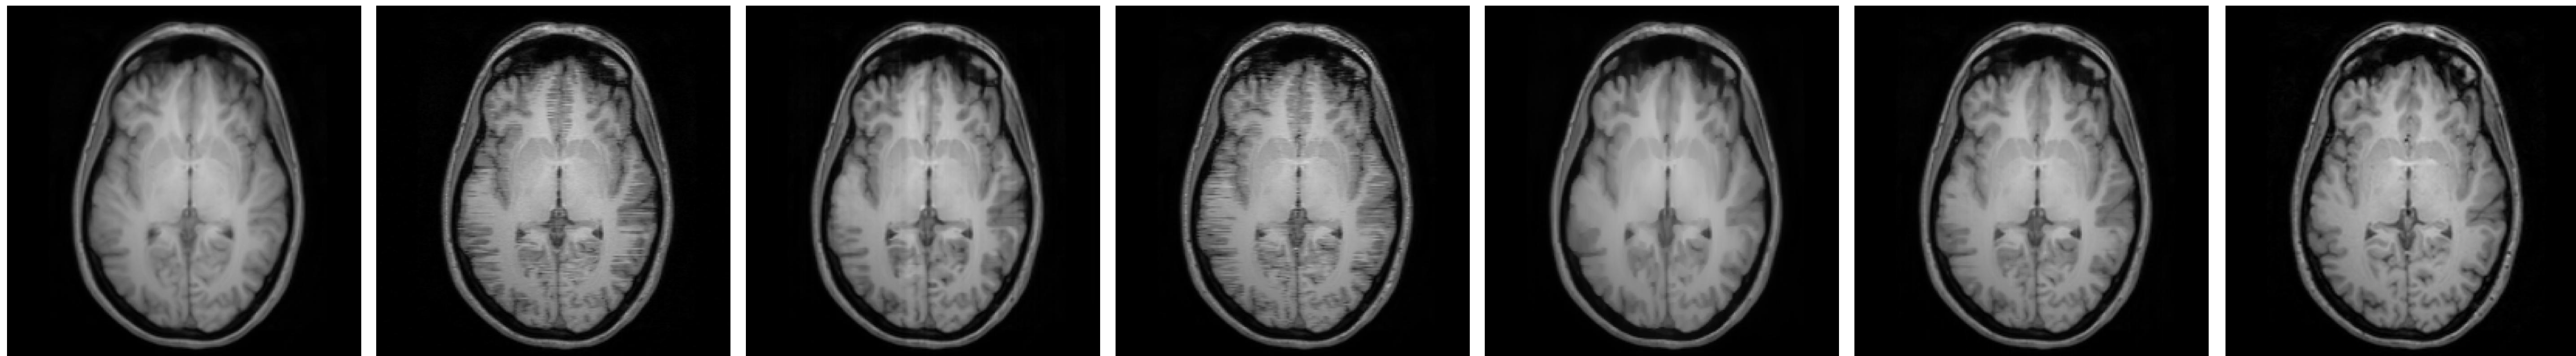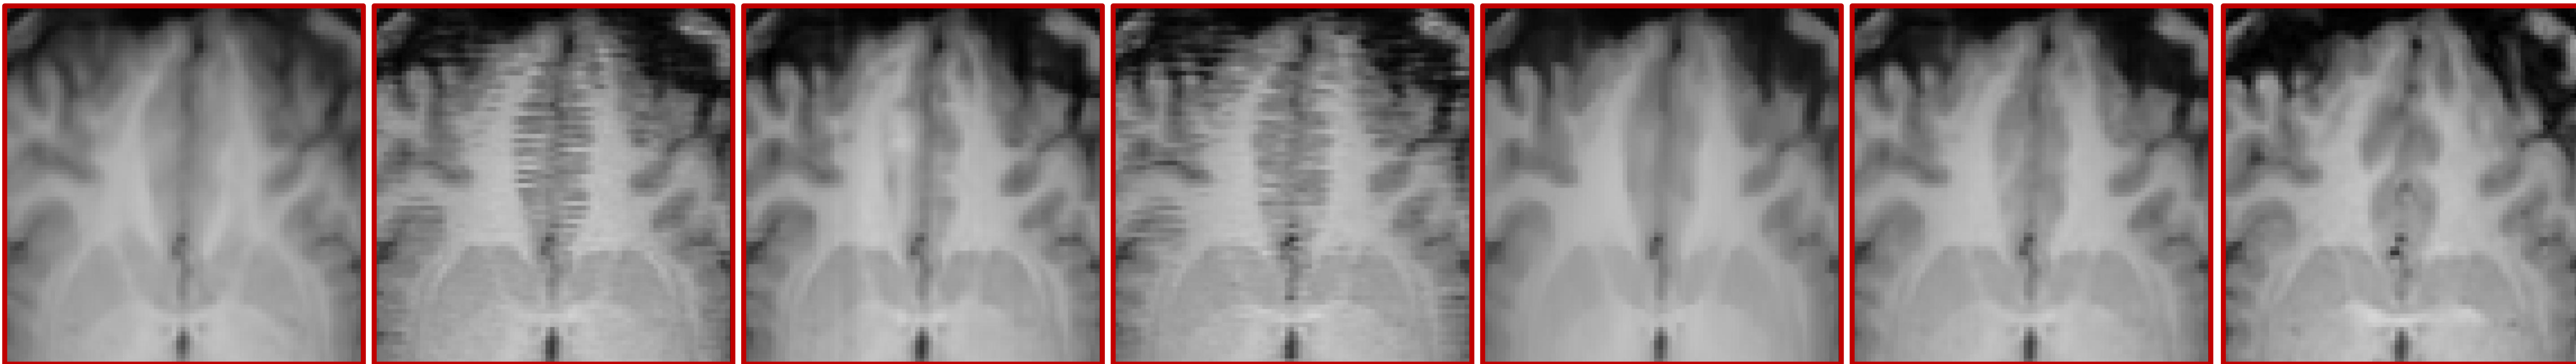

Sagittal

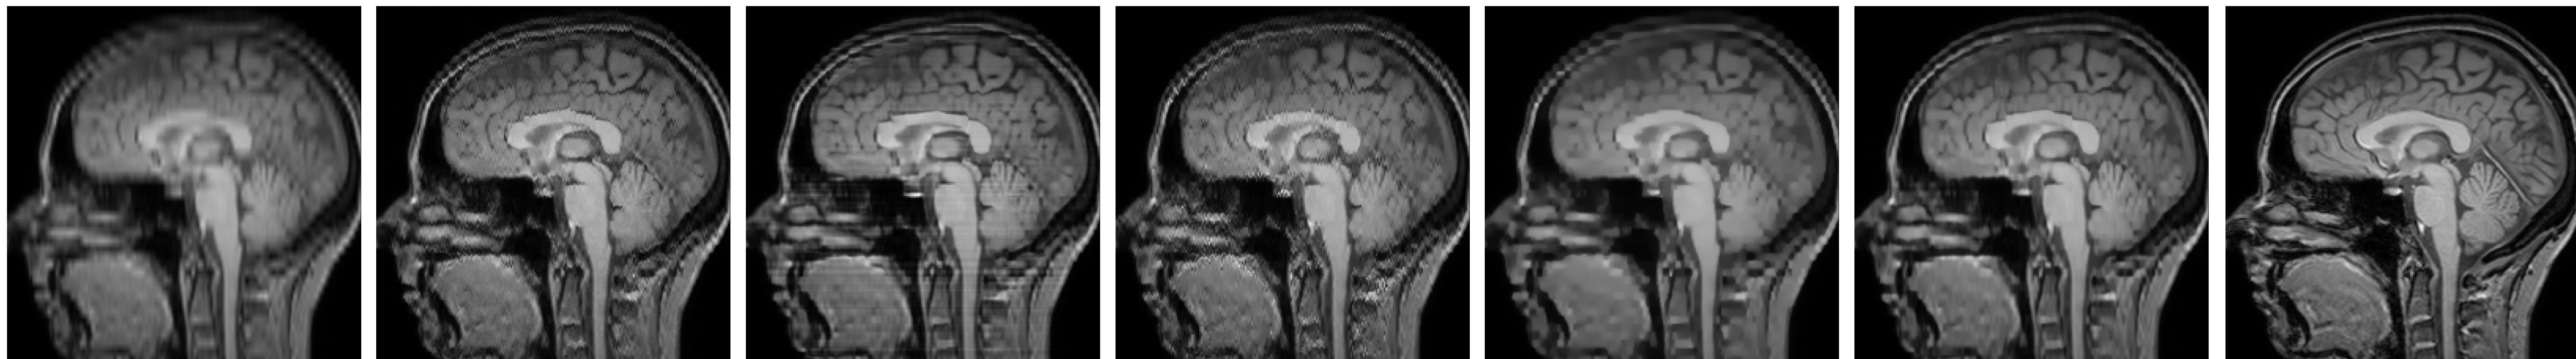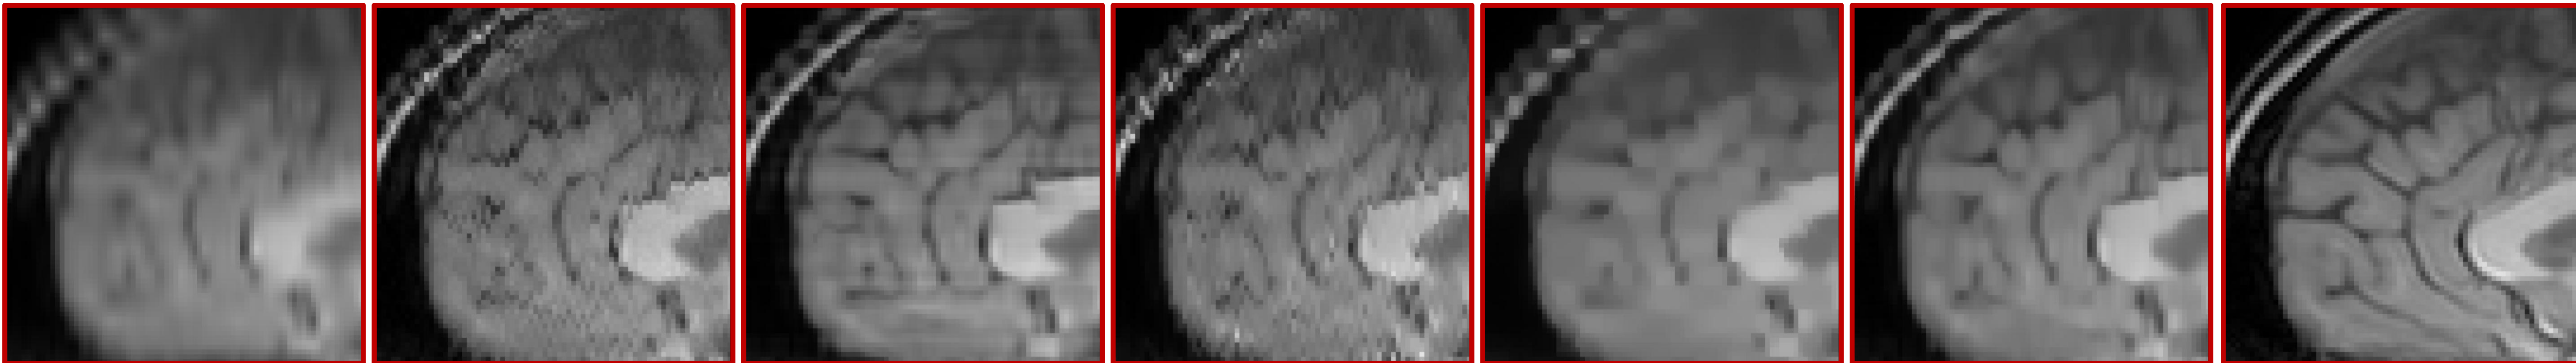

Coronal

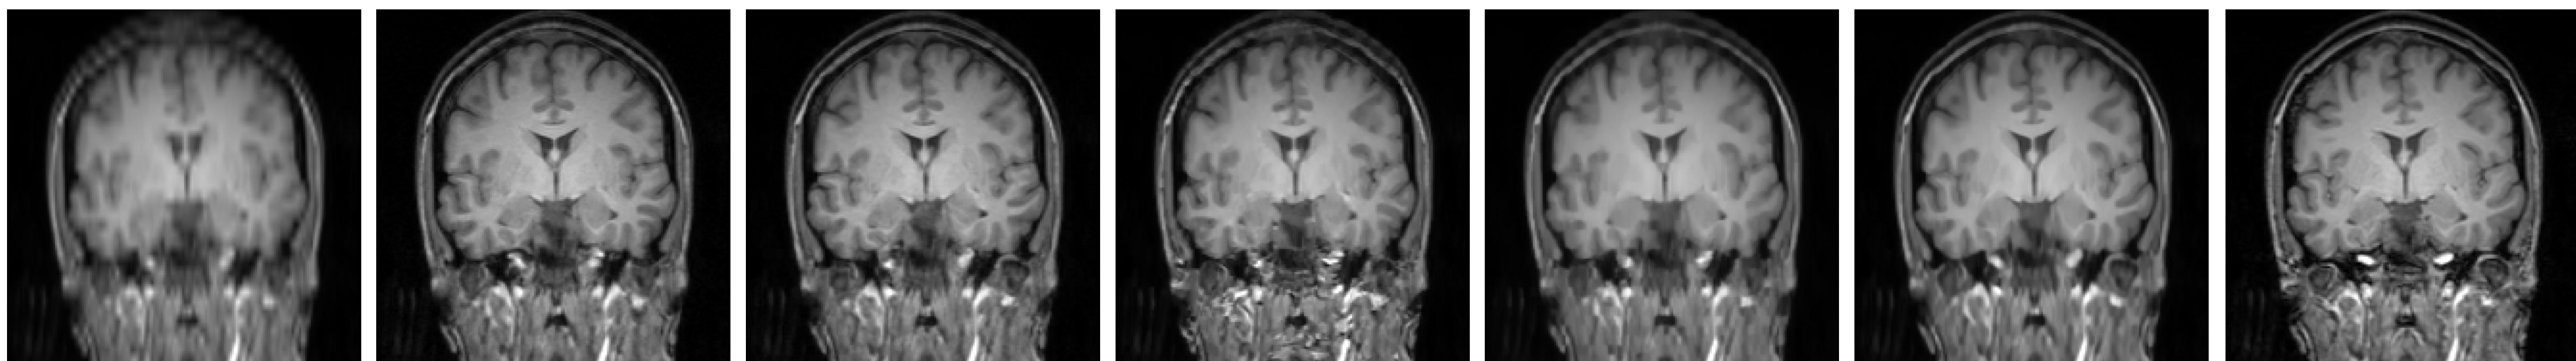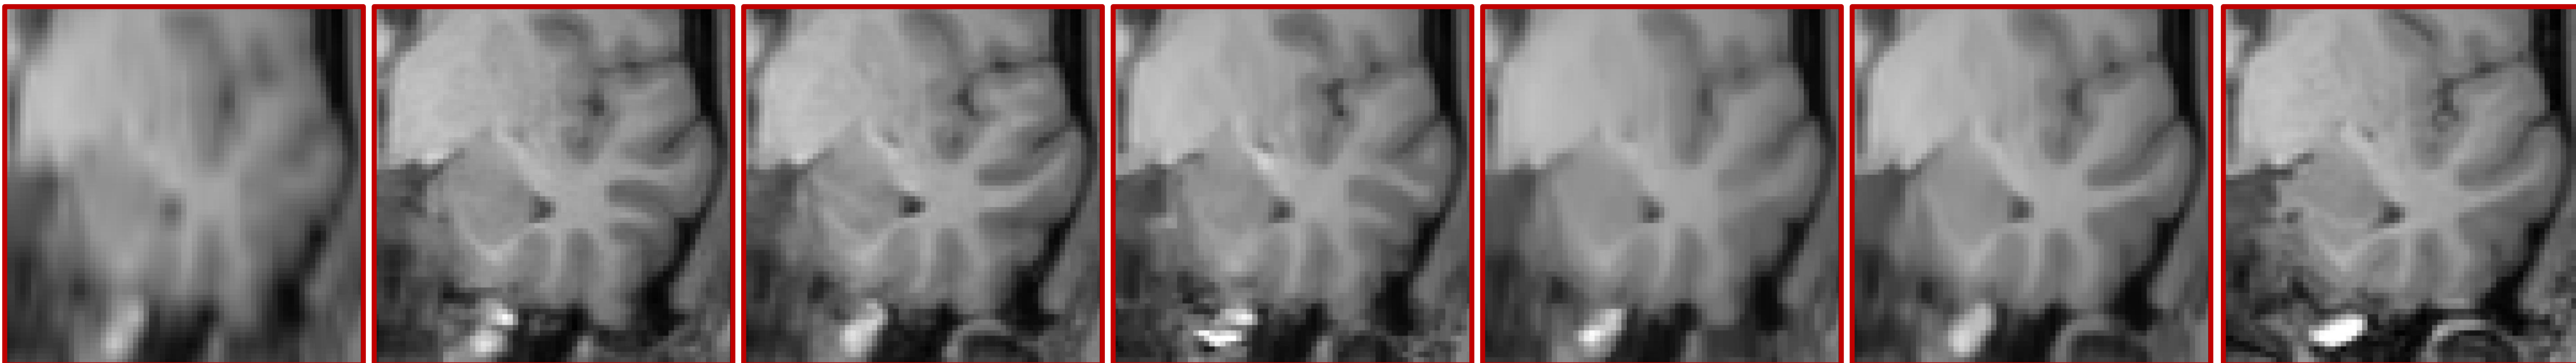

Cubic

DDNM

DDNM+ISCS

DDS

DDS+TV

DDS+ISCS

GT
